# Supplementary material for: Probabilistic Inverse Modeling: An Application in Hydrology
Source: arXiv:2210.06213 source file (2022-10-12)
Supplement: Supplementary file 1 [file appendix.tex]

\label{appendix}

\section{Reproducibility}
We use the KGSSL \cite{ghosh2021knowledge} code given \href{https://tinyurl.com/bdny7fk6}{here}. The daily-level CAMELS dataset used in this study is available \href{https://ral.ucar.edu/solutions/products/camels}{here}. The framework is built in \href{https://pytorch.org/}{PyTorch}, with the Bayes by Backprop module derived from \href{https://anaconda.org/conda-forge/blitz-bayesian-pytorch}{Blitz package}.

\textbf{Evaluating Model Performance:} The inverse model, $g_{\mathcal{S}}$, is trained on training set $\mathcal{S}$ such that, $g_S: [x_t^i, y_t^i] \rightarrow z_i$. In our case, training and test set are divided to test mod

\section{Proof of theorem 1}
\label{appendix:theorem1}

\begin{lemma}[\cite{kolter2008linear}]

For any real matrix $A$, the spectral norm of $v$ in decomposition $A = v^T v$, will be

\begin{equation*}
    ||v||^2_2 = \max_{||t||_2=1} ||vt||_2^2 
\end{equation*}

\begin{equation*}
    ||v||^2_2 = \max_{||t||_2=1} v^Hv t.t = \max_{||t||_2=1} t^T v^H v t = \lambda_1  
\end{equation*}

Here, $\lambda_1$ is the largest eigenvalue of $A$. Then, the normalized eigenvector of $\lambda_1$, $E_{\lambda_1}$ is of the form,

\begin{equation*}
    arg \max_{||t||_2=1} t^T v^Hvt = E_{\lambda_1}
\end{equation*}

\end{lemma}

\begin{theorem}
Let $g$ be our inverse model receiving training set $S$ as input such that, $g_S: [x_t^i, y_t^i] \rightarrow z_i$. A loss $\mathcal{L}_g$ for prediction function $g_S$ defined as $\frac{1}{t} \frac{1}{N} \sum_{i=1}^N \frac{1}{|z|} \sum_{j=1}^z w^j (z_i^j-\hat{z}_i^j)^2$ minimizes uncertainty $\sigma_S$ where $w^j$ corresponds with $E_{\lambda_1}$.

\end{theorem}

\begin{proof}

Let the penalty coefficient array be $w \in \mathbb{R}^z$. The formulation for guiding the learning to reduce uncertainty is,

\begin{equation}
   arg \min_{z_i^j} \frac{1}{N} \sum_{i=1}^N \frac{1}{|z|} \sum_{j=1}^z  w^j (z_i^j-\hat{z}_i^j)^2
\end{equation}

In order to obtain the optimal $w$ penalty coefficients to minimize overall uncertainty in response estimates over years, we use the epistemic uncertainty estimates in the response $\sigma \in \mathbb{R}^{N \times |z|}$, such that we have uncertainty estimate for each static characteristic in each training example. Let the eigenvalues of $\sigma$ be ordered as $\lambda_1 \ge \lambda_2 \ge ... \ge \lambda_z$. Utilizing the eigenvector and eigenvalues \cite{kolter2008linear} of $\sigma$, for 

\begin{equation}
    arg \max_{v \in R^Z, v^Tv \le 1} v^T \sigma v
\end{equation}

optimal $v$ is the eigenvector corresponding to $\lambda_1$, as stated in Lemma 1. The projection array $w = v \odot v$ will give us the optimal penalty coefficients.  Therefore, the uncertainty-based coefficients can be incorporated in the pseudo-inverse loss function as,

\begin{equation}
    \mathcal{L}'_{Inv} = \mathcal{L}_{Inv} + \frac{1}{t} \frac{1}{N} \sum_{i=1}^N \frac{1}{|z|} \sum_{j=1}^z w^j (z_i^j-\hat{z}_i^j)^2
\end{equation}

Here, $\sum_j v^Tv =1$, therefore, the penalized pseudo-inverse loss function also includes the convex sum of the loss from all static characteristics. Since the second term in this loss is smaller than the original pseudo-inverse loss, temperature scaling coefficient, $t$, can be included to change the scale of second loss term and can be learned as a hyper-parameter on the validation data set. 

\end{proof}

For static variables prediction problem, the dynamic behavior of the input data may act as natural adversarial noise affecting the robustness of the learned model. It may be conjectured, regularizing the loss to obtain lower epistemic uncertainty estimates mitigates the effect of dynamic adversarial perturbations. In our inverse model, which is a fully trained, overparameterized Bayesian neural network (BNN), averaging under the posterior leads to reduced effect of perturbations. BNNs act as ensemble of NNs that, in large data limit, have gradient of loss orthogonal to the data manifold \cite{carbone2020robustness}.

\section{Source of Uncertainty}
\label{appendix:sourceofunc}

In our experiments, we develop a robust representation learning framework that relies on a non-deterministic approximation of encoded representations and a principled objective formulation to learn observational and inductive bias. This framework not only benefits from accurate reconstruction of driver-response variables, but also relies on learning representation based on corrupted / noisy input source. Different components of the framework can be made non - deterministic by perturbing the weights of different layers in the network \cite{blundell2015weight}. Depending on the component, the source of uncertainty varies and so does the epistemic uncertainty in our posterior prediction function. Table~\ref{tab:sourceofunc} shows the model performance for different variations of the KGSSL framework with different sources of uncertainty. The different variants propagate uncertainty differently through the loss terms. With a probabilistic encoder module, uncertainty can be propagated through all the loss terms, allowing us to obtain uncertainty in reconstruction of static characteristics and also the dynamic characteristics. In the probabilistic model, the increased number of trainable parameters leads to slower learning (10\% increase in training time complexity). While a deterministic model may be able to learn a complex, rich parameterization, the probabilistic model provides an added advantage of measuring the uncertainty in such a model approximation.

\begin{table*}[]
    \tiny
    \centering
    \begin{tabular}{|p{3cm}|p{2.2cm}|p{1.4cm}|p{2.2cm}|p{1.8cm}|p{1cm}|p{1.5cm}|}
    \toprule
          Source of Uncertainty & Impacted Loss Term & Validation MSE & Reconstruction Loss & Contrastive Loss & Inverse Loss & Static Uncertainty\\
          \hline
          Deterministic & - & 0.2646 & 1.9265 & 0.1473 & 0.2630 & - \\
          Decoder & Reconstruction & 0.2992 & 3.7056 & 0.1588 & 0.2791 & 0.0 \\
          Encoder & All & 0.2791 & 1.9864 & 0.1480 & 0.2750 & 0.0013 \\
          Static Reconstruction Module (First Linear Layer) & Inverse & 0.2917 & 1.9479 & 0.1591 & 0.2884 & 0.0039 \\
          Static Reconstruction Module (Second Linear Layer) & Inverse & 0.2950 & 2.1156 & 0.1548 & 0.2909 & 0.0038 \\
          Reconstruction Module (Last Linear Layer) & Contrastive & 0.3083 & 2.0448 & 0.1678 & 0.3050 & 0.0 \\
          \bottomrule
    \end{tabular}
    \caption{Different sources of uncertainty lead to different prediction model performance. Using a probabilistic encoder enables uncertainty estimation corresponding to the three loss terms.}
    \label{tab:sourceofunc}
\vspace{-10pt}
\end{table*}

Here, epistemic uncertainty ($\sigma_i$) can be measured as the standard error in prediction estimates over repeated trials. The standard error is the variability arising in the estimates due to uncertainty arising from imperfect data or model miss-specification. As can be seen in Table~\ref{tab:sourceofunc}, the probabilistic encoder based model yields the lowest inverse loss (static feature reconstruction MSE) among the probabilistic variants and also the lowest uncertainty value on the validation data set. For the purpose of further experiments in this work, we focus on the probabilistic encoder based model.

% Further analysis can benefit in the understanding of how uncertainty varies in the absence of some of the loss terms. Some early experiments in this direction have been summarized in the appendix section \textcolor{red}{include}.

\section{Temporal Variance in Static Variables}
\label{appendix:similarity}

\begin{figure}[h]

\centering
\begin{tabular}{c|c}
% \toprule

 \subcaptionbox{\label{fig:unc-similarity-matrices} Clean Training Data Results \vspace{5pt} }{\includegraphics[scale=0.1]{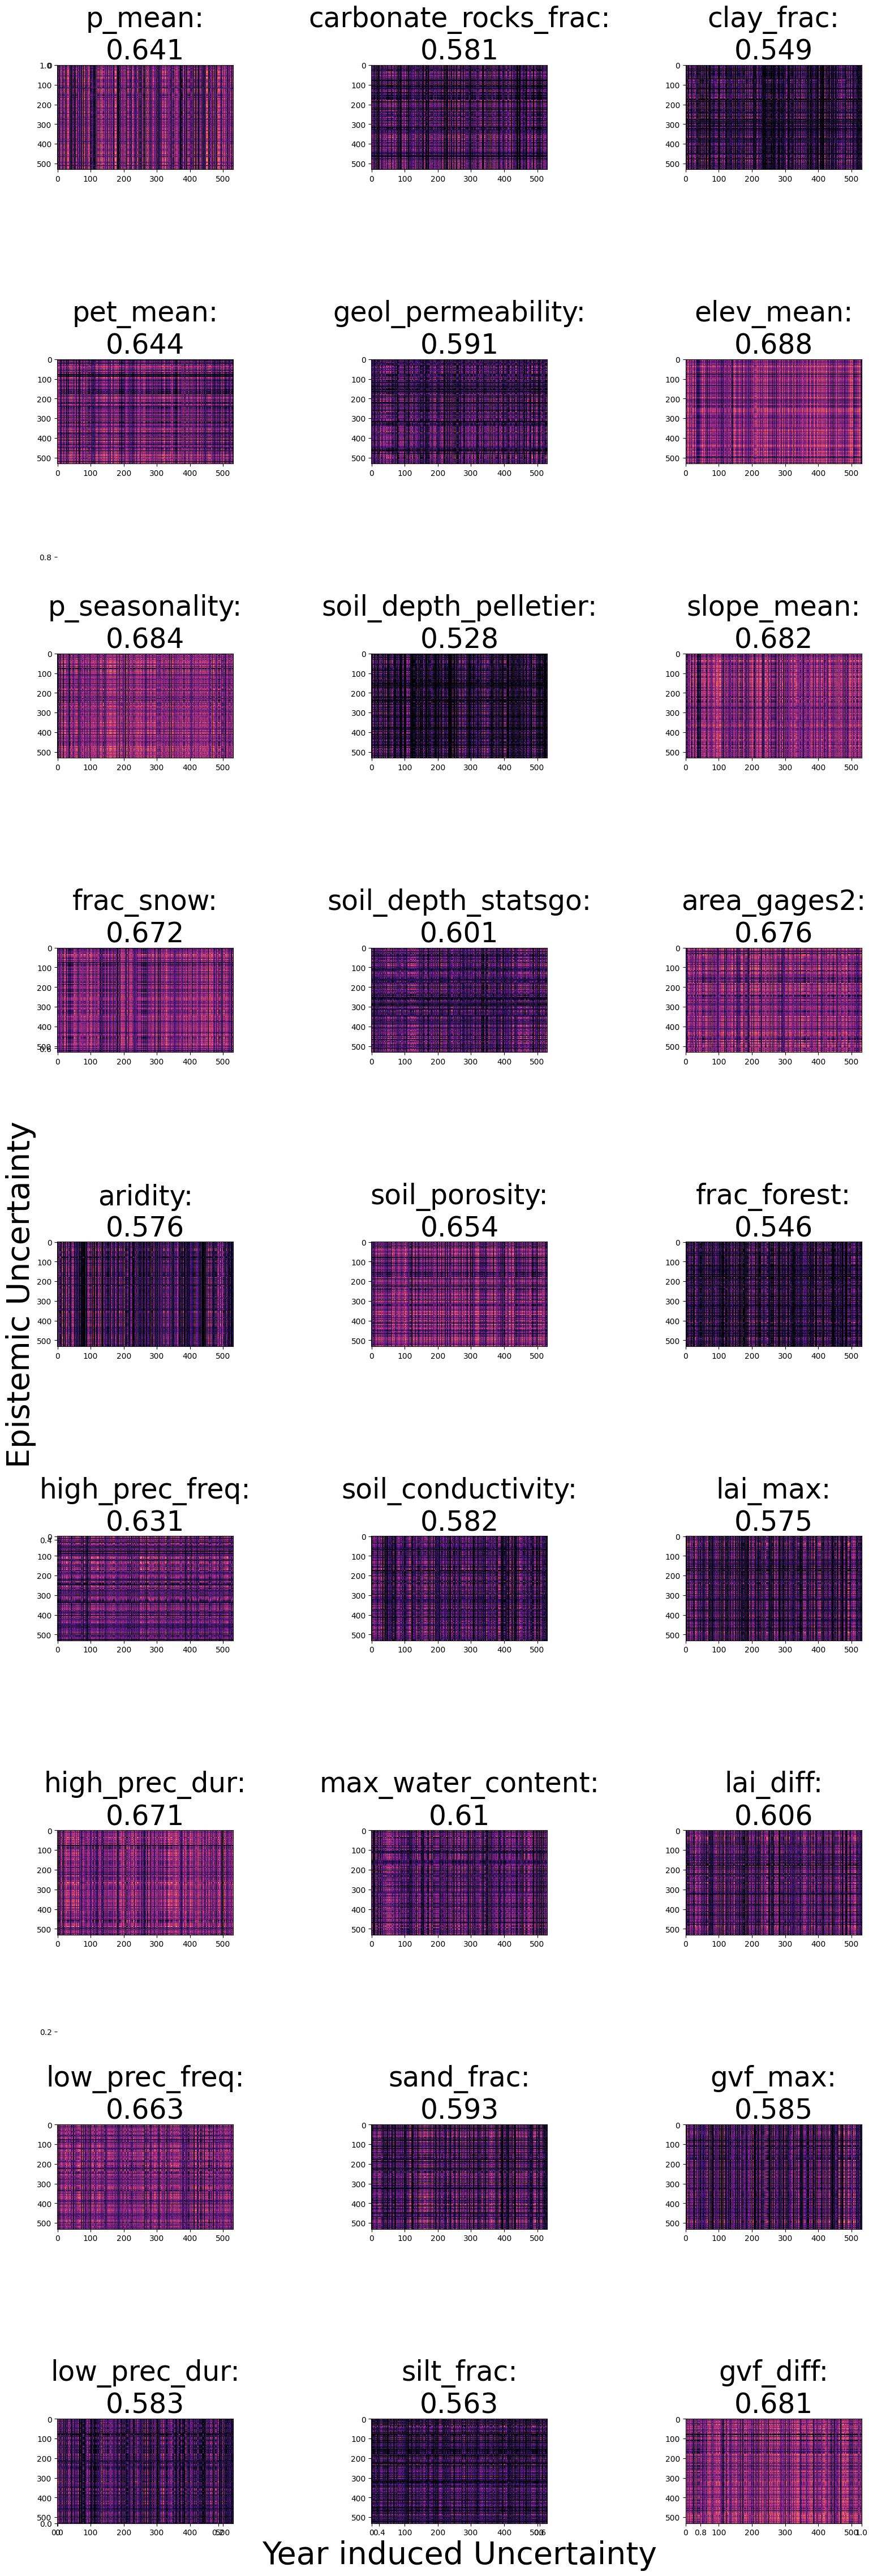}} &
%  \subcaptionbox{\label{fig:corr-unc-50-01} 50\% training data perturbed with standard deviation 0.1 \vspace{5pt} }{\includegraphics[scale=0.1]{images/results/corrupt/unc/{}_basin_test_similarity_unc_vanilla_50_0.1.png}} &
 \subcaptionbox{\label{fig:corr-unc-50-5} 50\% training data perturbed with standard deviation 5 \vspace{5pt} }{\includegraphics[scale=0.1]{images/results/corrupt/unc/{}_basin_test_similarity_unc_vanilla_50_5.png}} \\ % &
%  \subcaptionbox{\label{fig:corr-unc-50-5-minmax} 50\% training data perturbed with standard deviation 5 (Uncertainty Based Learning) \vspace{5pt} }{\includegraphics[scale=0.1]{images/results/corrupt/unc/{}_basin_test_similarity_unc_minmax_50_5.png}} \\
% \hline

\end{tabular}
\caption{Similarity between uncertainty in static characteristic estimates over the years (x-axis) and epistemic uncertainty (y-axis). Correlation mentioned in plot titles with variable name.. The similarity between uncertainty over years and epistemic uncertainty also varies by the amount of perturbation.}
\label{fig:corrupt-50-similarity}

\vspace{-10pt}
\end{figure}

Uncertainty arises since the inverse model overlooks the invariant behavior in observed static characteristics while estimating them from dynamical variables. This causes the static characteristics estimates to vary considerably over days and years. This \textit{uncertainty over time} ($unc_i$) is related to the overall uncertainty due to insufficient input data ($\sigma_i$). The association between the two uncertainty estimates is measured for all basins in Sub-figure~\ref{fig:unc-similarity-matrices} as, $\text{Correlation}_i = corr( unc_i, \sigma_i)$.

As both $unc_i$ and $\sigma_i$ are measures of variance in our static characteristic estimates, a more confident model would have smaller correlation (regardless of how the model is performing in terms of the  bias in the estimates). This is because a naive functional approximation of static characteristics from temporally varying variables increases the uncertainty in the model. This increased variability also allows for a bigger bandwidth for the response estimates to vary in over time, increasing the $unc_i$ values as well. Therefore, we are able to notice a positive correlation between epistemic uncertainty and uncertainty arising from varying behavior of the static characteristic reconstructions. Darker regions indicate lower levels of correlation. We can notice higher levels of correlation between the two uncertainties for the weather based and geo-morphology based static features. Previous studies have indicated that in the forward model, climate variables may be more important in predicting streamflow than soil based factors \cite{stein2021climate, li2022regionalization}. In the inverse modeling, lesser signals to learn from may lead to worse reconstructions for soil based factors ( visible in the high bias in (Figure~\ref{fig:det-and-prob-predictions}) and the varying levels of similarity for different variables ( Figure~\ref{fig:unc-similarity-matrices}). This may also point towards different scope of improvement for different variables based on the measured uncertainty. In sub-section~\ref{sec:results-ubl}, we penalize highly uncertain representations to improve the confidence in entity characteristic reconstructions.

% \begin{figure}[h]

% \centering
% \begin{tabular}{c}
% % \toprule

% \includegraphics[scale=0.13]{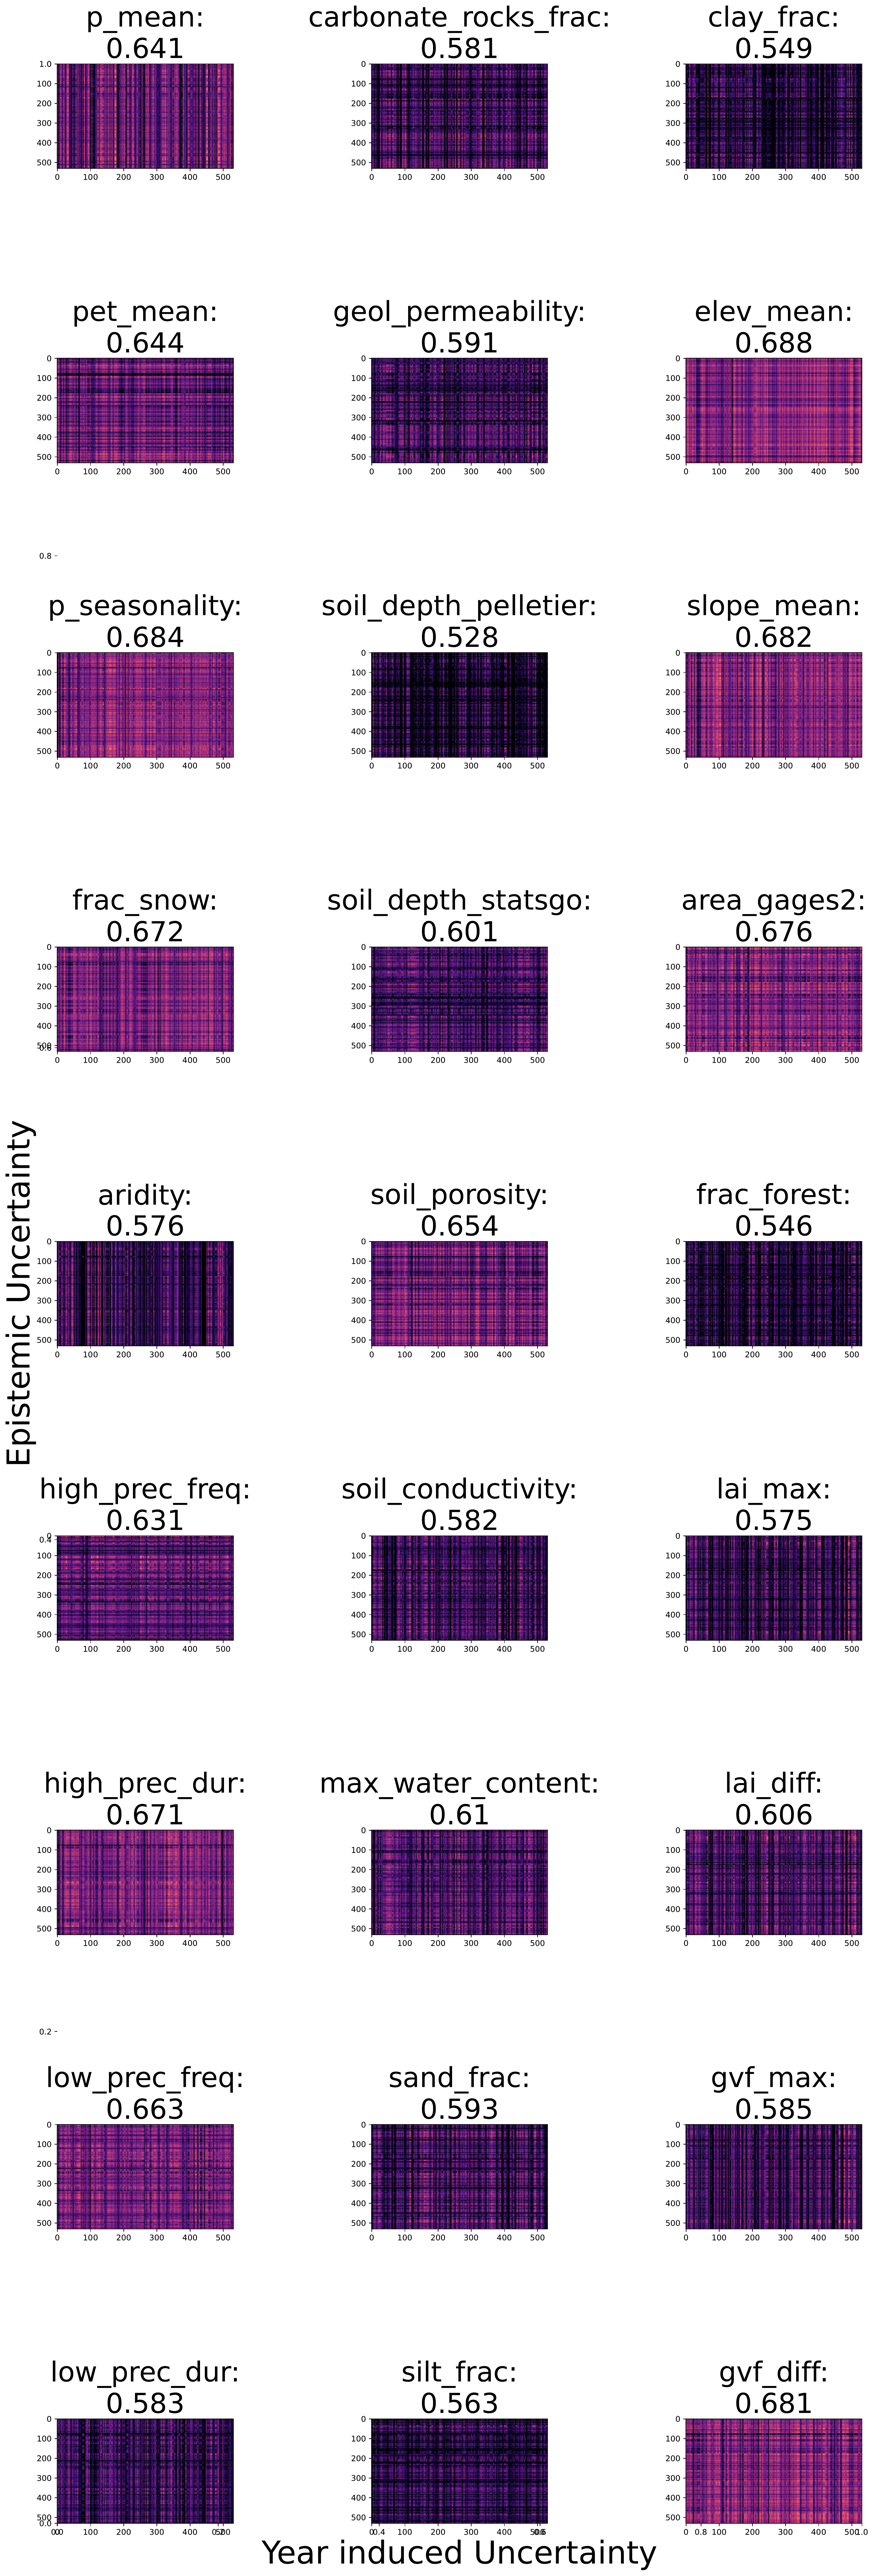} \\

% \end{tabular}
% \caption{Similarity between uncertainty in static characteristic estimates over the years (x-axis) and epistemic uncertainty (y-axis) under uncertainty based penalties. Correlation mentioned in plot titles with variable name.}
% \label{fig:unc-similarity-matrices}

% \vspace{-10pt}
% \end{figure}

\section{Figures}

We predict static characteristics for all 531 river basins in the test period (Figure~\ref{fig:det-and-prob-predictions}). These predictions are made from KGSSL and probabilistic encoder based KGSSL. The black line represents the golden standard for accurate predictions. Predictions are plotted on the Y-axis while the CAMELS provided estimates are plotted on the X-axis. Blue solid dots lying on the black line indicate accurate predictions. The yellow error bars represent the standard deviation in these reconstructions over the whole test period. For both the models, the bias and standard error in the soil-based feature reconstructions is the highest (second row in each of the sub-figures). In further analysis, we focus on reducing this variance in reconstructions over time.

\begin{figure*}[h]

\centering
\begin{tabular}{c}
% \toprule

 \subcaptionbox{\label{fig:deterministic_model_scatterplot} Deterministic KGSSL \vspace{5pt} }{\includegraphics[scale=0.15]{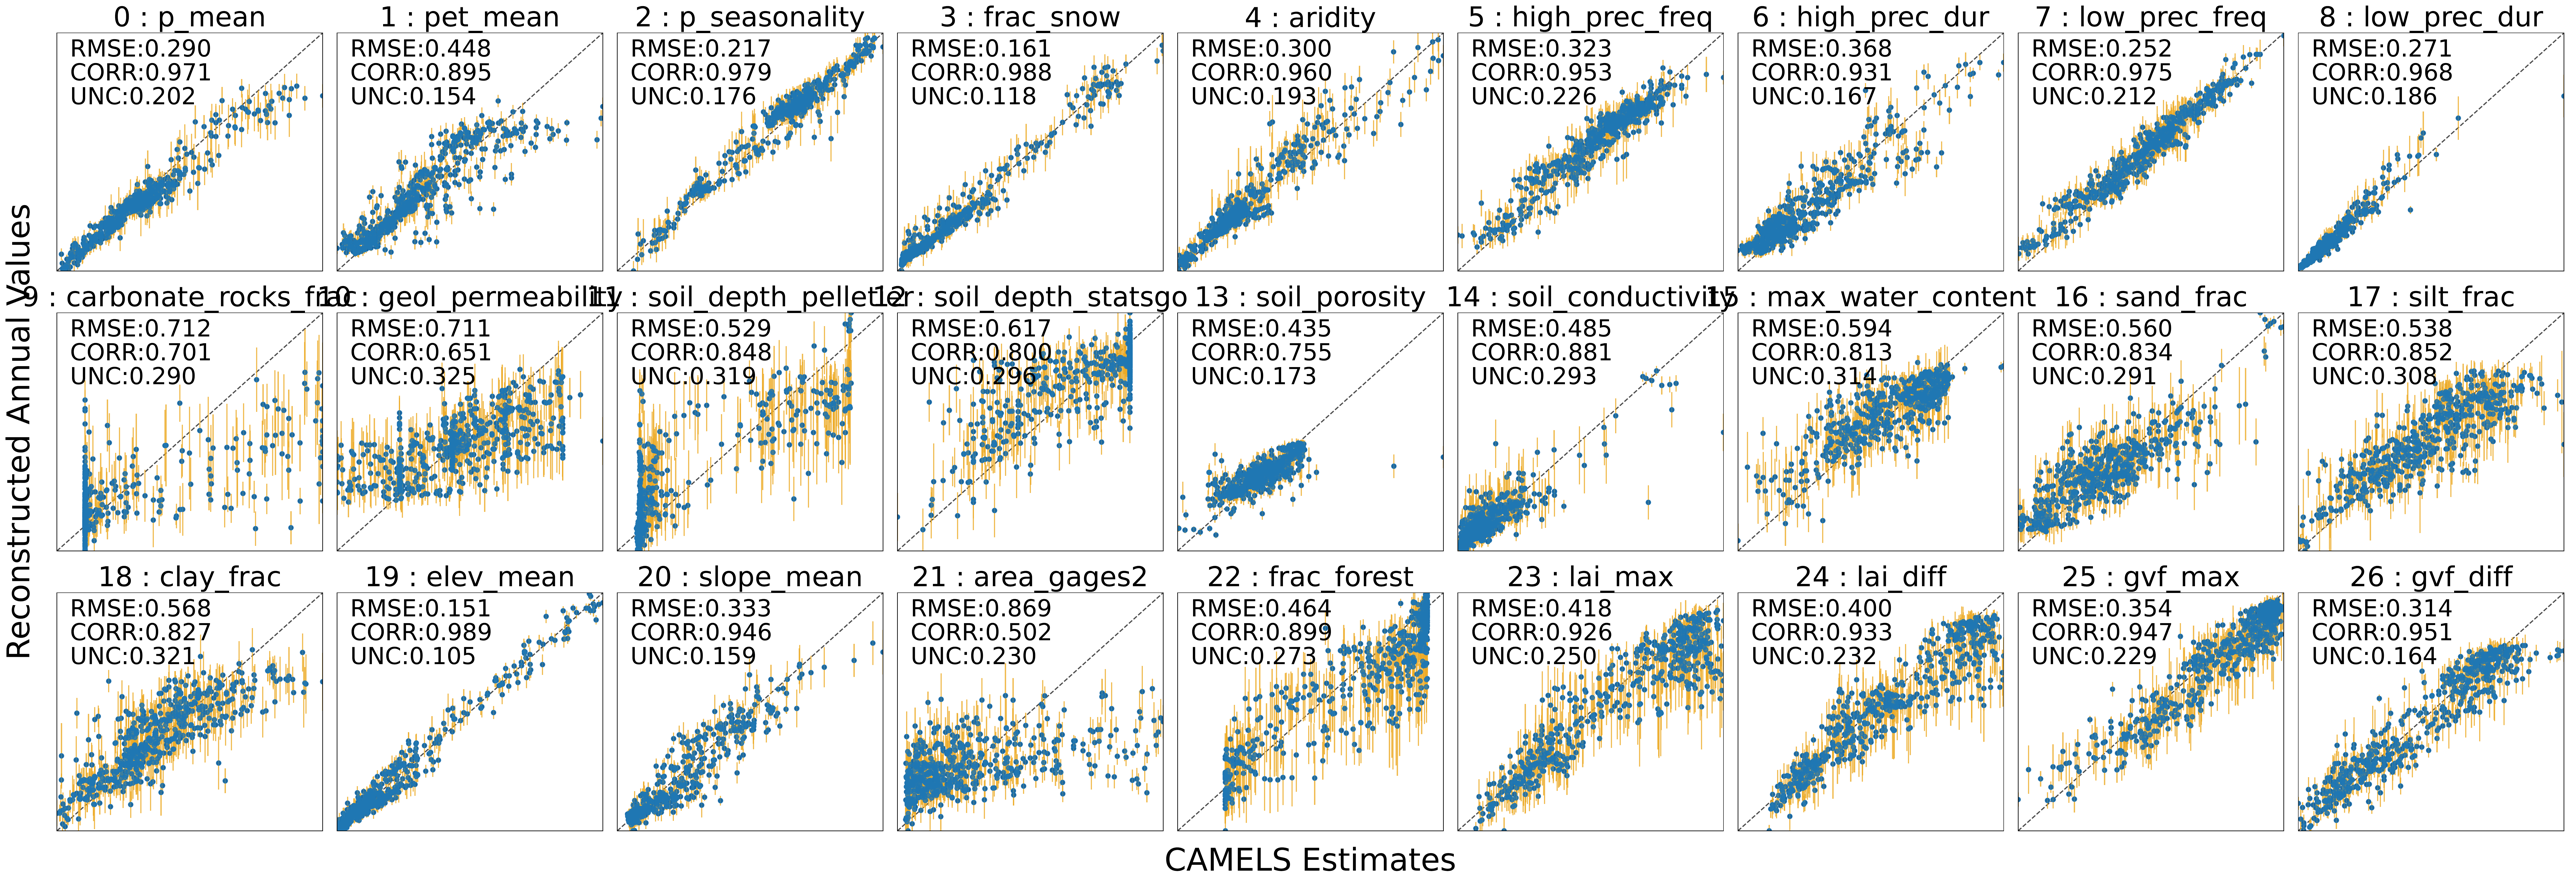}} \\
  \subcaptionbox{\label{fig:probabilistic_model_scatterplot} Probabilistic Encoder based KGSSL \vspace{5pt} }{\includegraphics[scale=0.15]{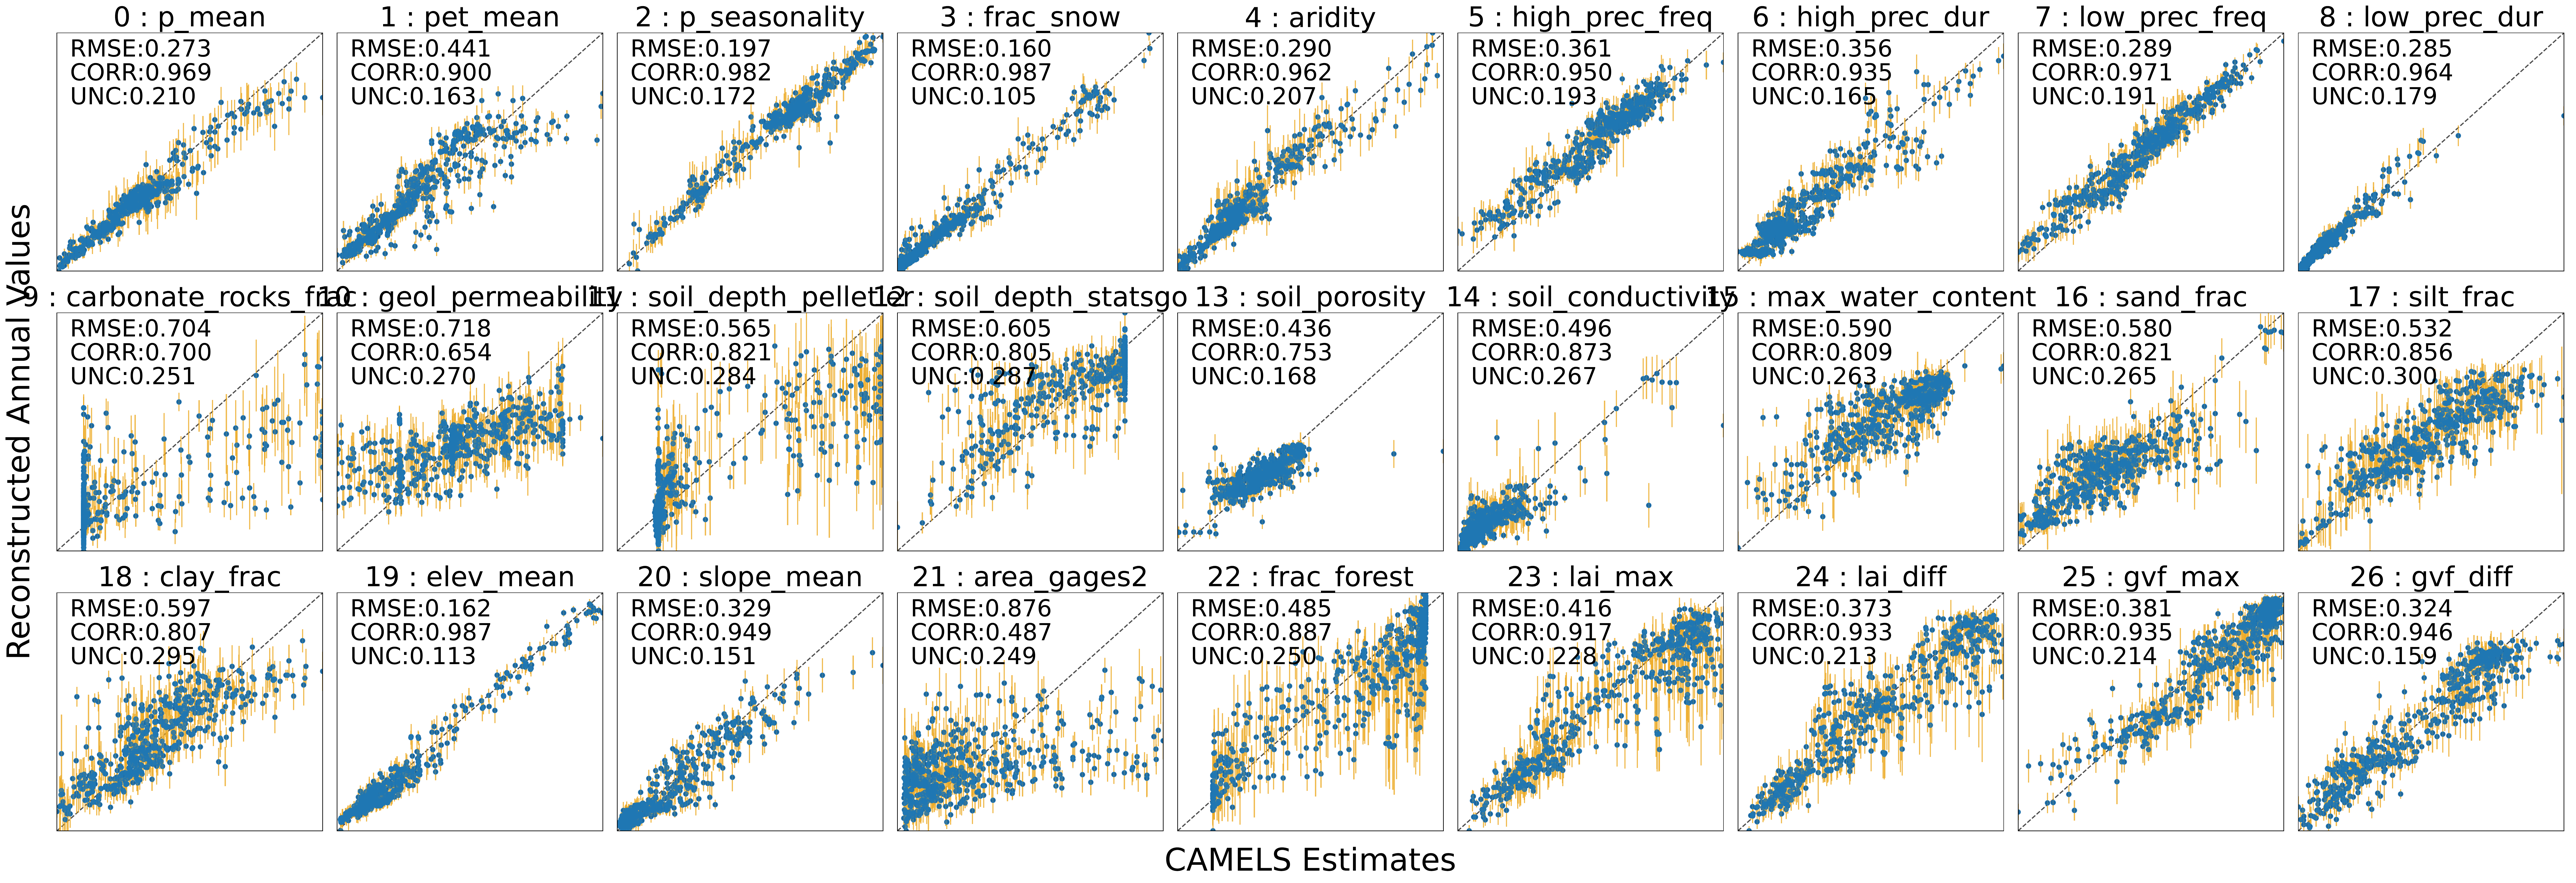}} \\
% \hline

\end{tabular}
\caption{The static characteristic estimates can be compared with the observed values for the 531 basins. Basins falling along the black dotted line represent accurate estimation. The yellow error bars represent variability in estimates over the years in the test dataset.}
\label{fig:det-and-prob-predictions}

\vspace{-10pt}
\end{figure*}

\section{Miscellaneous Figures}

% \subsection{Sources of Uncertainty}

% \begin{figure*}[]
%     \centering
%     \includegraphics[width=0.7\linewidth]{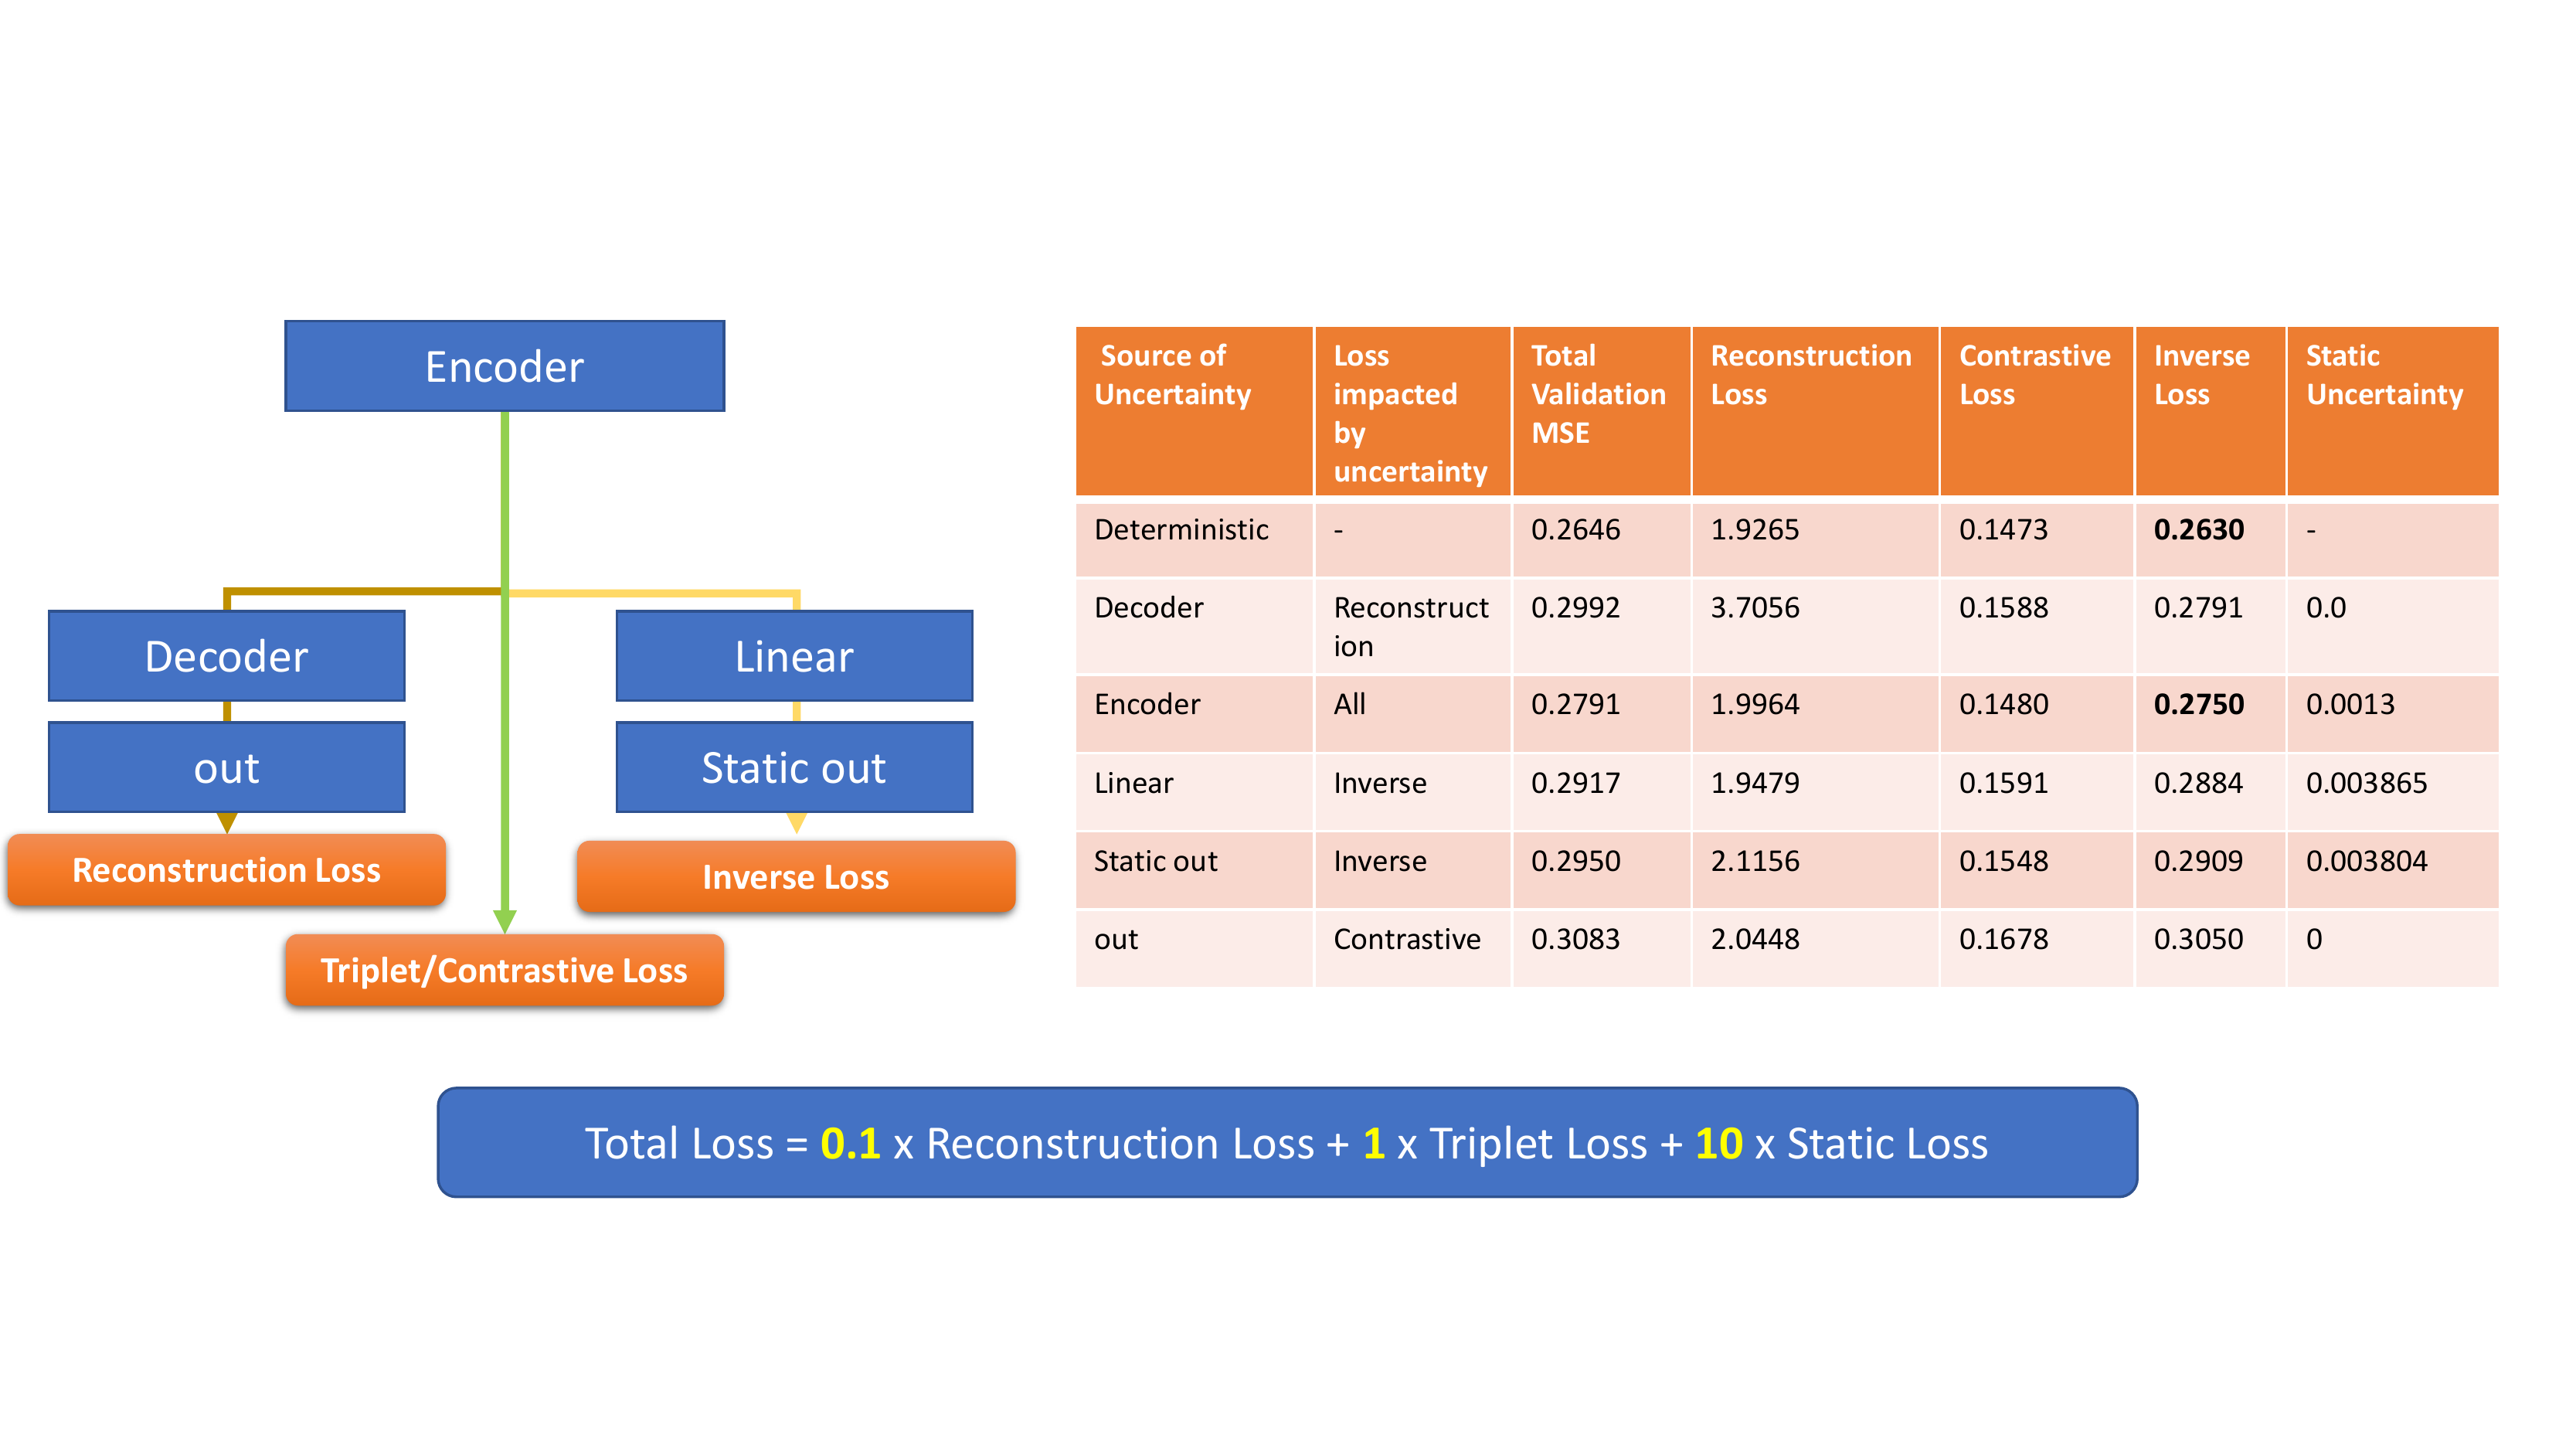}
%     \caption{Validation MSE loss values with different sources of uncertainty in architecture of KGSSL Framework. \textcolor{red}{use draw.io or affinity}}
%     \label{fig:validation_unc}
% \end{figure*}

% \subsection{Deterministic Model Estimate vs Observed}

% \begin{figure*}[t!]
%     \centering
%     \includegraphics[width=0.7\linewidth]{images/results/clean_data/scatterplots/ATT_NL_0_basin_test.pdf}
%     \caption{The static characteristic estimates can be compared with the observed values for the 531 basins. Basins falling along the black dotted line represent accurate estimation. The yellow error bars represent variability in estimates over the years in the test dataset.}
%     \label{fig:deterministic_model_scatterplot}
% \end{figure*}

% \subsection{Probabilistic Model Estimate vs Observed}

% \begin{figure*}[t!]
%     \centering
%     \includegraphics[width=0.7\linewidth]{images/results/clean_data/scatterplots/ATT_NL_3_basin_test.pdf}
%     \caption{The static characteristic estimates from the probabilistic model can be compared with the observed values for the 531 basins. Basins falling along the black dotted line represent accurate estimation. The yellow error bars represent variability in estimates over the years in the test dataset.}
%     \label{fig:probabilistic_model_scatterplot}
% \end{figure*}

\begin{figure*}[h]
    \centering
    \includegraphics[width=0.7\linewidth]{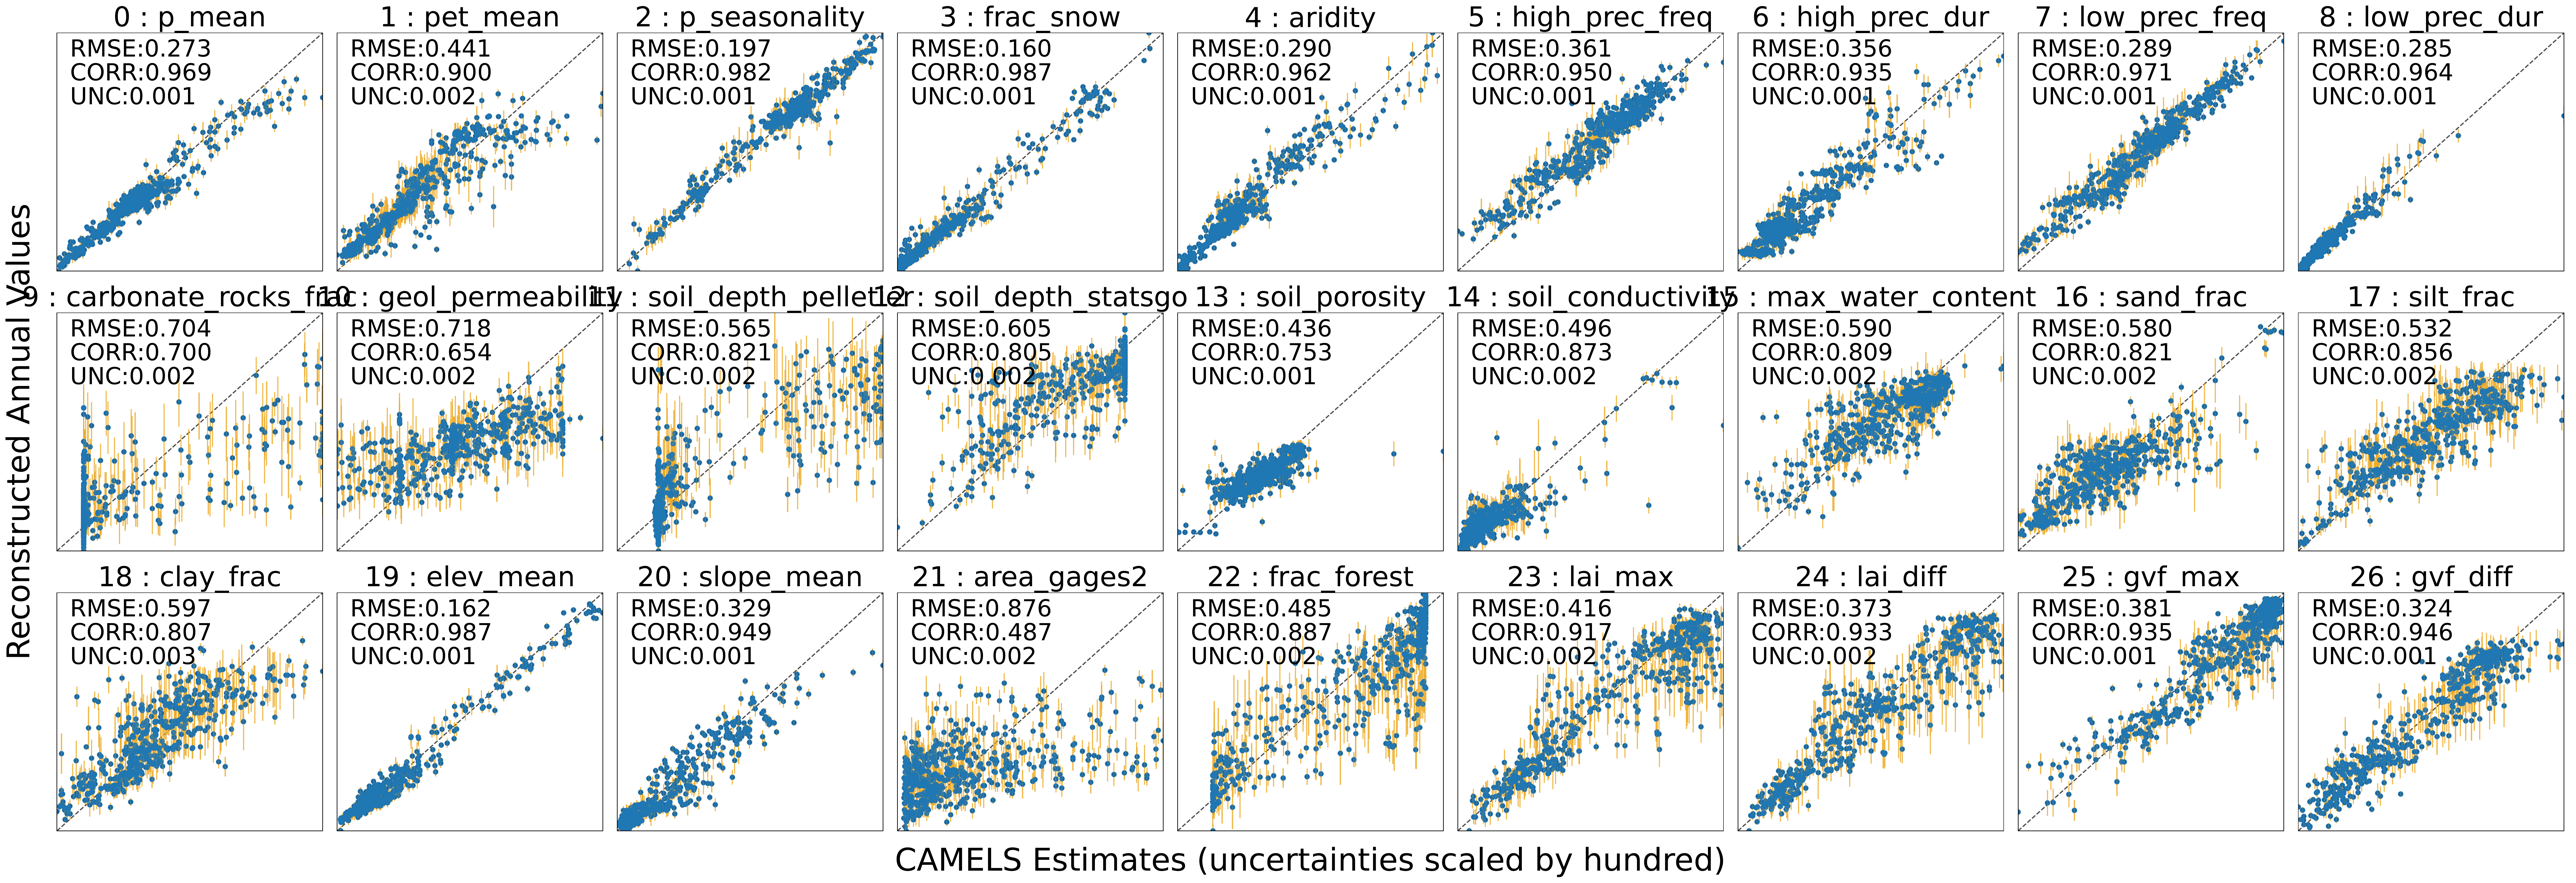}
    \caption{Probabilistic Model Estimate vs Observed, errorbar is epistemic uncertainty: The static characteristic estimates from the probabilistic model can be compared with the observed values for the 531 basins. Basins falling along the black dotted line represent accurate estimation. The yellow error bars represent the epistemic uncertainty in the test set.}
    \label{fig:probabilistic_model_scatterplot_epistemicuncertainty}
\end{figure*}

\begin{figure*}[h]
    \centering
    \includegraphics[width=0.7\linewidth]{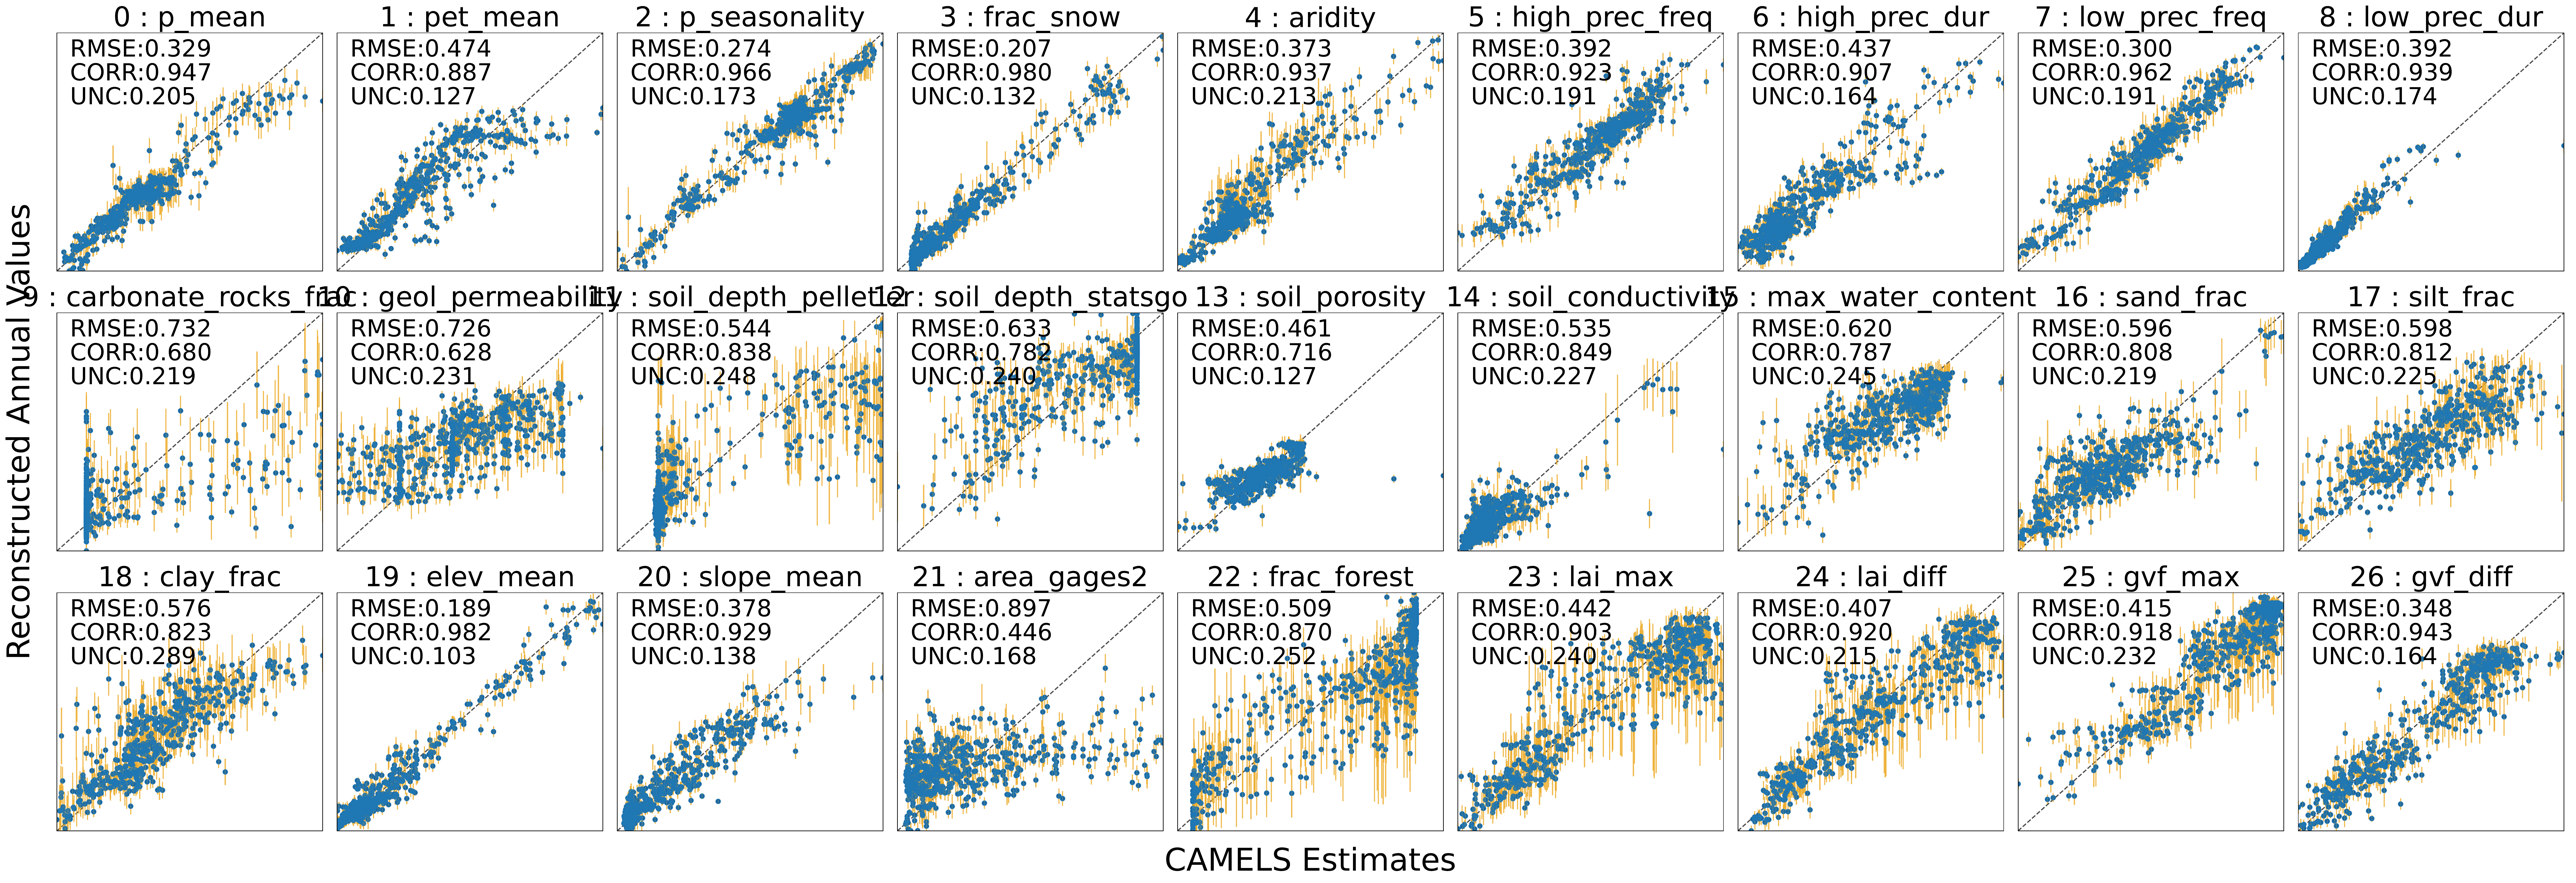}
    \caption{Min-Max Uncertainty based Optimization: The static characteristic estimates from the min-max uncertainty optimized probabilistic model can be compared with the observed values for the 531 basins. Basins falling along the black dotted line represent accurate estimation. The yellow error bars represent variability in estimates over the years in the test dataset.}
    \label{fig:probabilistic_model_scatterplot_minmax}
\end{figure*}

\begin{figure*}[h]
    \centering
    \includegraphics[width=0.3\linewidth]{images/results/uncertainty/ATT_NL_3_basin_test_similarity_unc_minmax.pdf}
    \caption{Correlation between uncertainty over years and epistemic uncertainty, uncertainty based learning: Similarity between uncertainty in static characteristic estimates over the years (x-axis) and epistemic uncertainty (y-axis) under uncertainty based penalties. Correlation mentioned in plot titles with variable name.}
    \label{fig:probabilistic_model_uncertainty_correlation}
\end{figure*}

\begin{figure*}[h]
    \centering
    \includegraphics[width=0.7\linewidth]{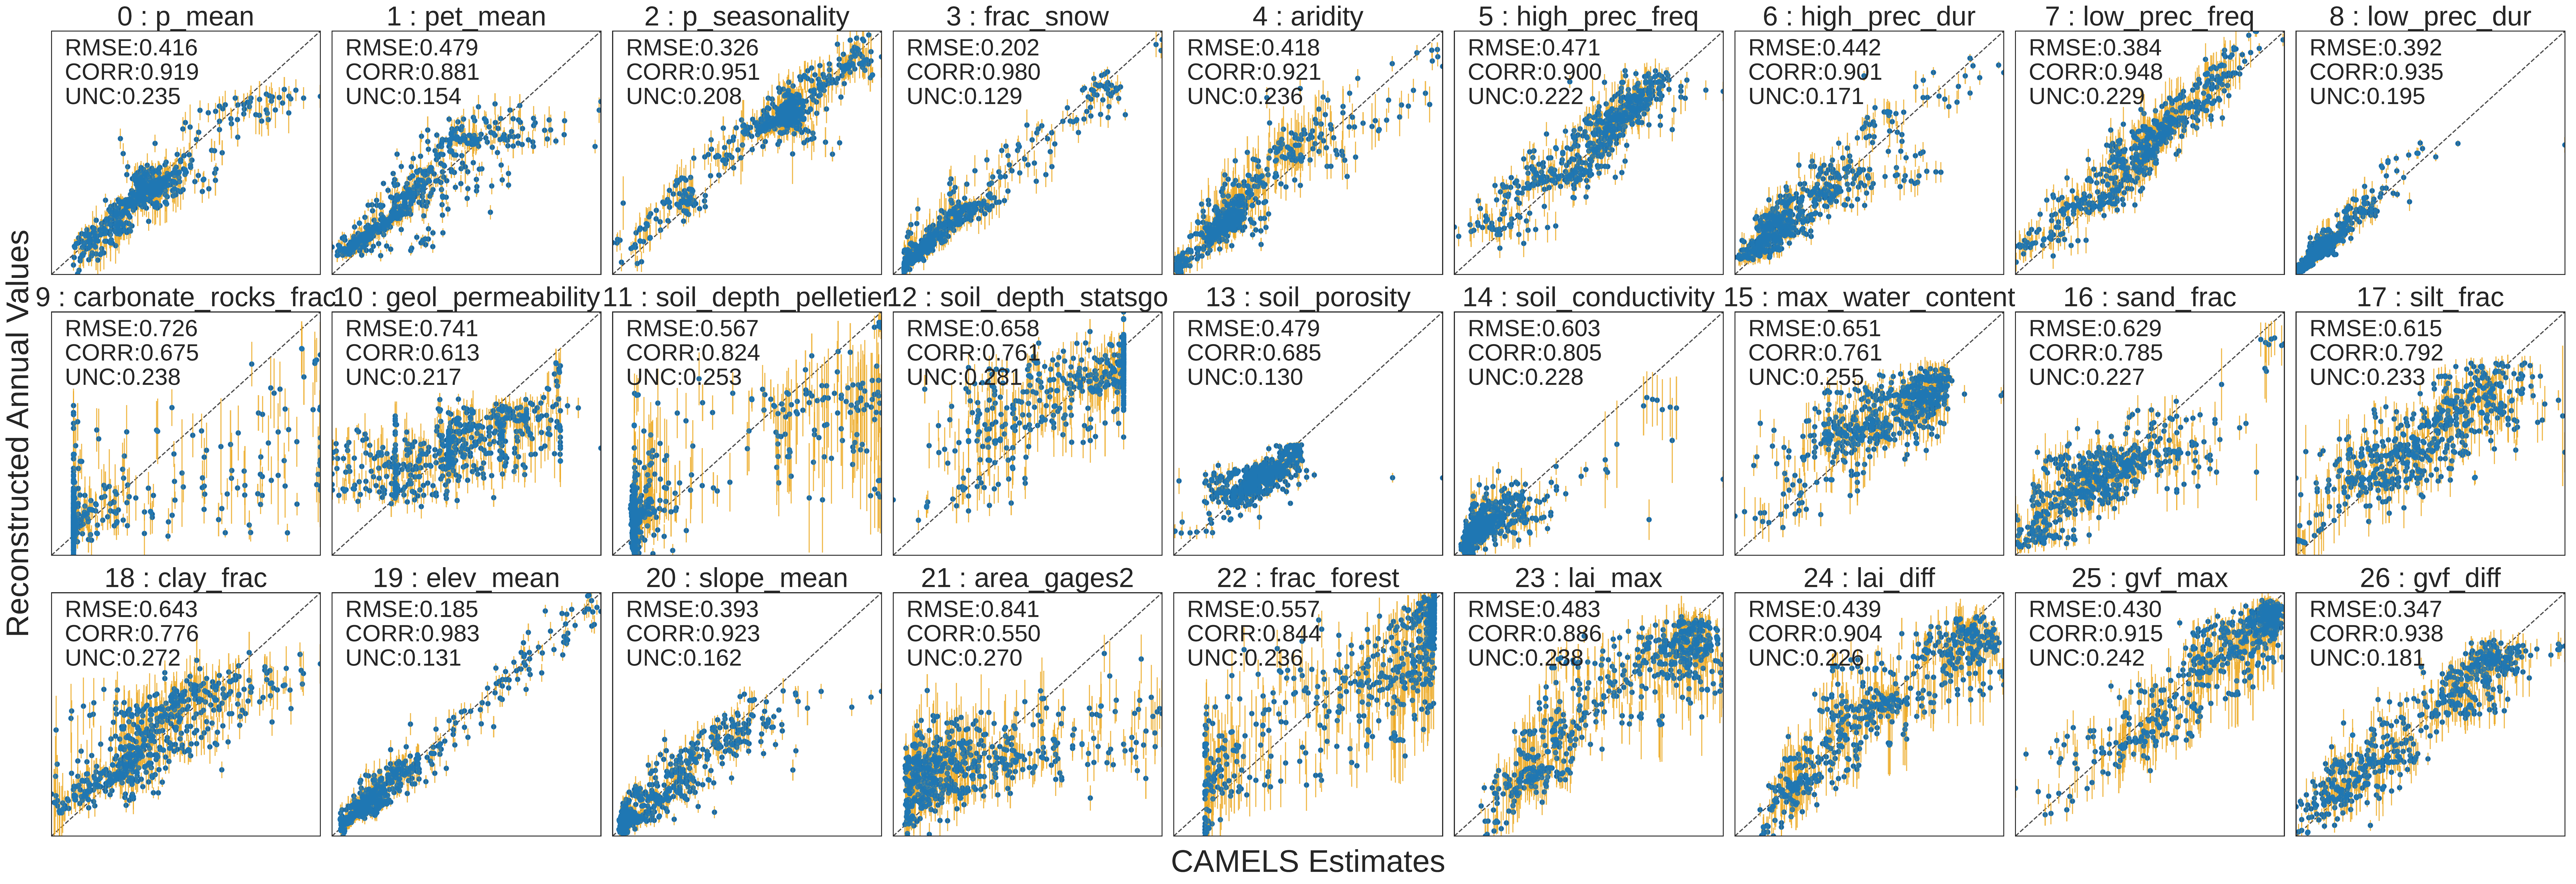}
    \caption{Min-Max MSE based Optimization: The static characteristic estimates from the min-max mse optimized probabilistic model can be compared with the observed values for the 531 basins. Basins falling along the black dotted line represent accurate estimation. The yellow error bars represent variability in estimates over the years in the test dataset.}
    \label{fig:probabilistic_model_scatterplot_minmax_mse}
\end{figure*}

\begin{figure*}[h]
    \centering
    \includegraphics[width=0.3\linewidth]{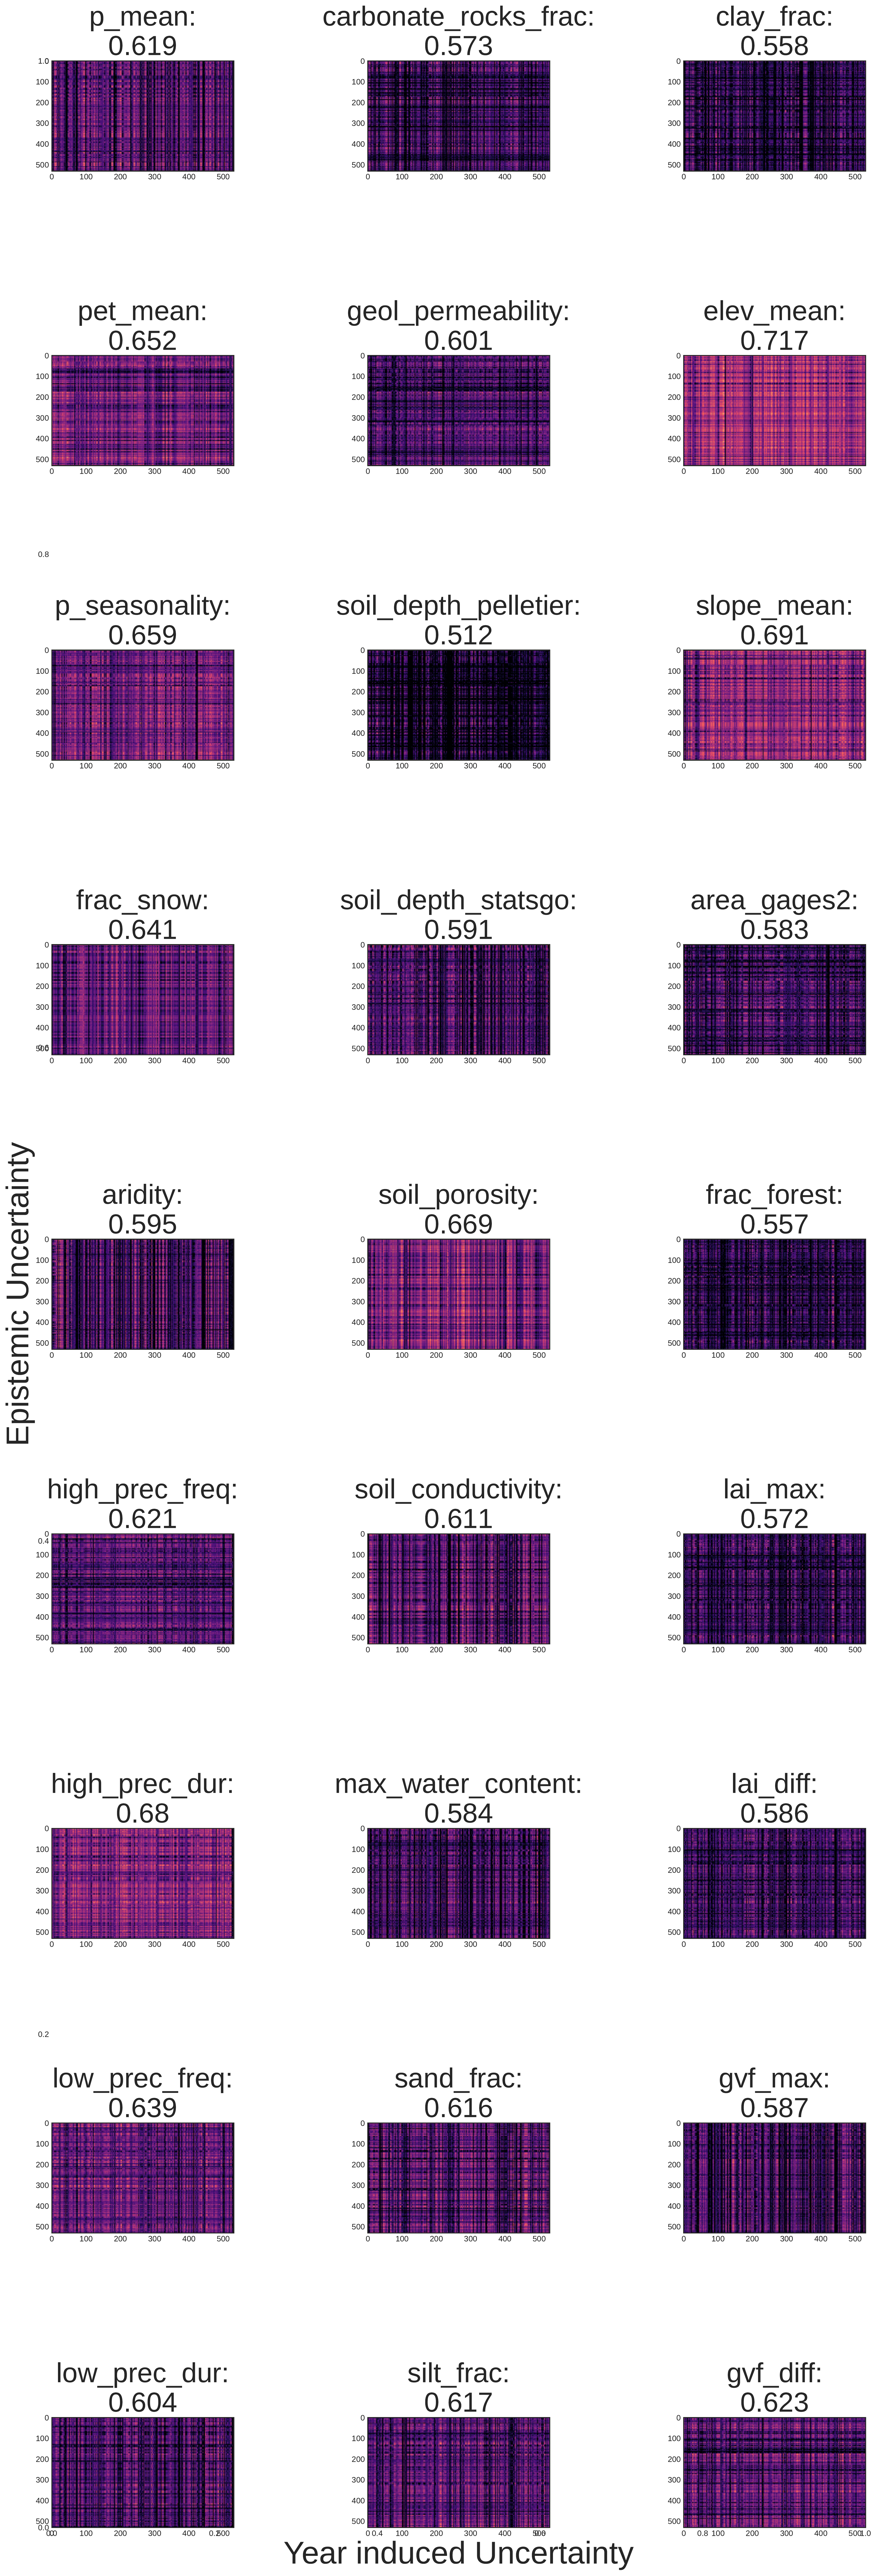}
    \caption{Correlation between uncertainty over years and epistemic uncertainty, mse based penalties: Similarity between uncertainty in static characteristic estimates over the years (x-axis) and epistemic uncertainty (y-axis) under mse based penalties. Correlation mentioned in plot titles with variable name.}
    \label{fig:probabilistic_model_uncertainty_correlation_minmax_mse}
\end{figure*}
